# Supplementary material for: Maximizing Alignment with Minimal Feedback: Efficiently Learning Rewards for Visuomotor Robot Policy Alignment
Source: arXiv:2412.04835 source file (2024-12-06)
Supplement: Supplementary file 1 [file appendix.tex]

\section{Appendix}
\label{app:appendix}

\subsection{Optimal Transport Based Reward}
\label{app:OT}

\rb{\subsection{Attention Map for \rapl and \rlhf}

In Figure~\ref{fig:attention_map} we visualize the attention map with a novel use of \textit{linear permutation} and \textit{kernel inflation} \citep{xu2022image2point}. Specifically, we use channel-averaged 2D feature map (\textit{i.e.,} activation map) as our attention map \citep{xu2020squeezesegv3}. Different from previous works that operate 2D feature maps, our approach utilizes a linear mapping $\mathcal{W} \in \mathcal{R}^{C_{in} \times C_{out}}$ on a 1D feature, which is average-pooled from a 2D feature $\mathcal{F}_{2D} \in \mathcal{R}^{C_{in} \times H \times W}$. Mathematically, the procedure can be formulated as
\begin{equation}
    \hat{\mathcal{F}}_{1D} = \frac{\mathcal{W}^T \times \sum_i^{H \times W}\mathcal{F}_{2D}^i}{H \times W}
\end{equation}
where $\hat{\mathcal{F}}_{1D} \in \mathcal{R}^{C_{out} \times 1}$ is the aligned features from our proposed RAPL by $\mathcal{W} \in \mathcal{R}^{C_{in} \times C_{out}}$. Inspired by \cite{xu2022image2point}, we can inflate the 1D linear mapping $\mathcal{W} \in \mathcal{R}^{C_{in} \times C_{out}}$ into 2D and keep the kernel size as 1, \textit{i.e.}, $\mathcal{W} \in \mathcal{R}^{C_{in} \times C_{out}} \rightarrow \mathcal{W}_{inflate} \in \mathcal{R}^{C_{in} \times C_{out} \times 1 \times 1}$. Then above equation can be equally represented as 
\begin{equation}
     \hat{\mathcal{F}}_{2D}  = \mathcal{W}_{inflate}^T \times \mathcal{F}_{2D}, 
     \hat{\mathcal{F}}_{1D} = \frac{\sum_i^{H \times W}\hat{\mathcal{F}}^i_{2D}}{H \times W}
\end{equation}
We average the $\hat{\mathcal{F}}_{2D} \in \mathcal{R}^{C_{out} \times H \times W}$ in channel dimension, and visualize the output as our attention map. A visualization of the full process is shown in Figure~\ref{fig:attention_map_method}.}

\begin{figure*}[h]
    \centering
    \includegraphics[width=\textwidth]{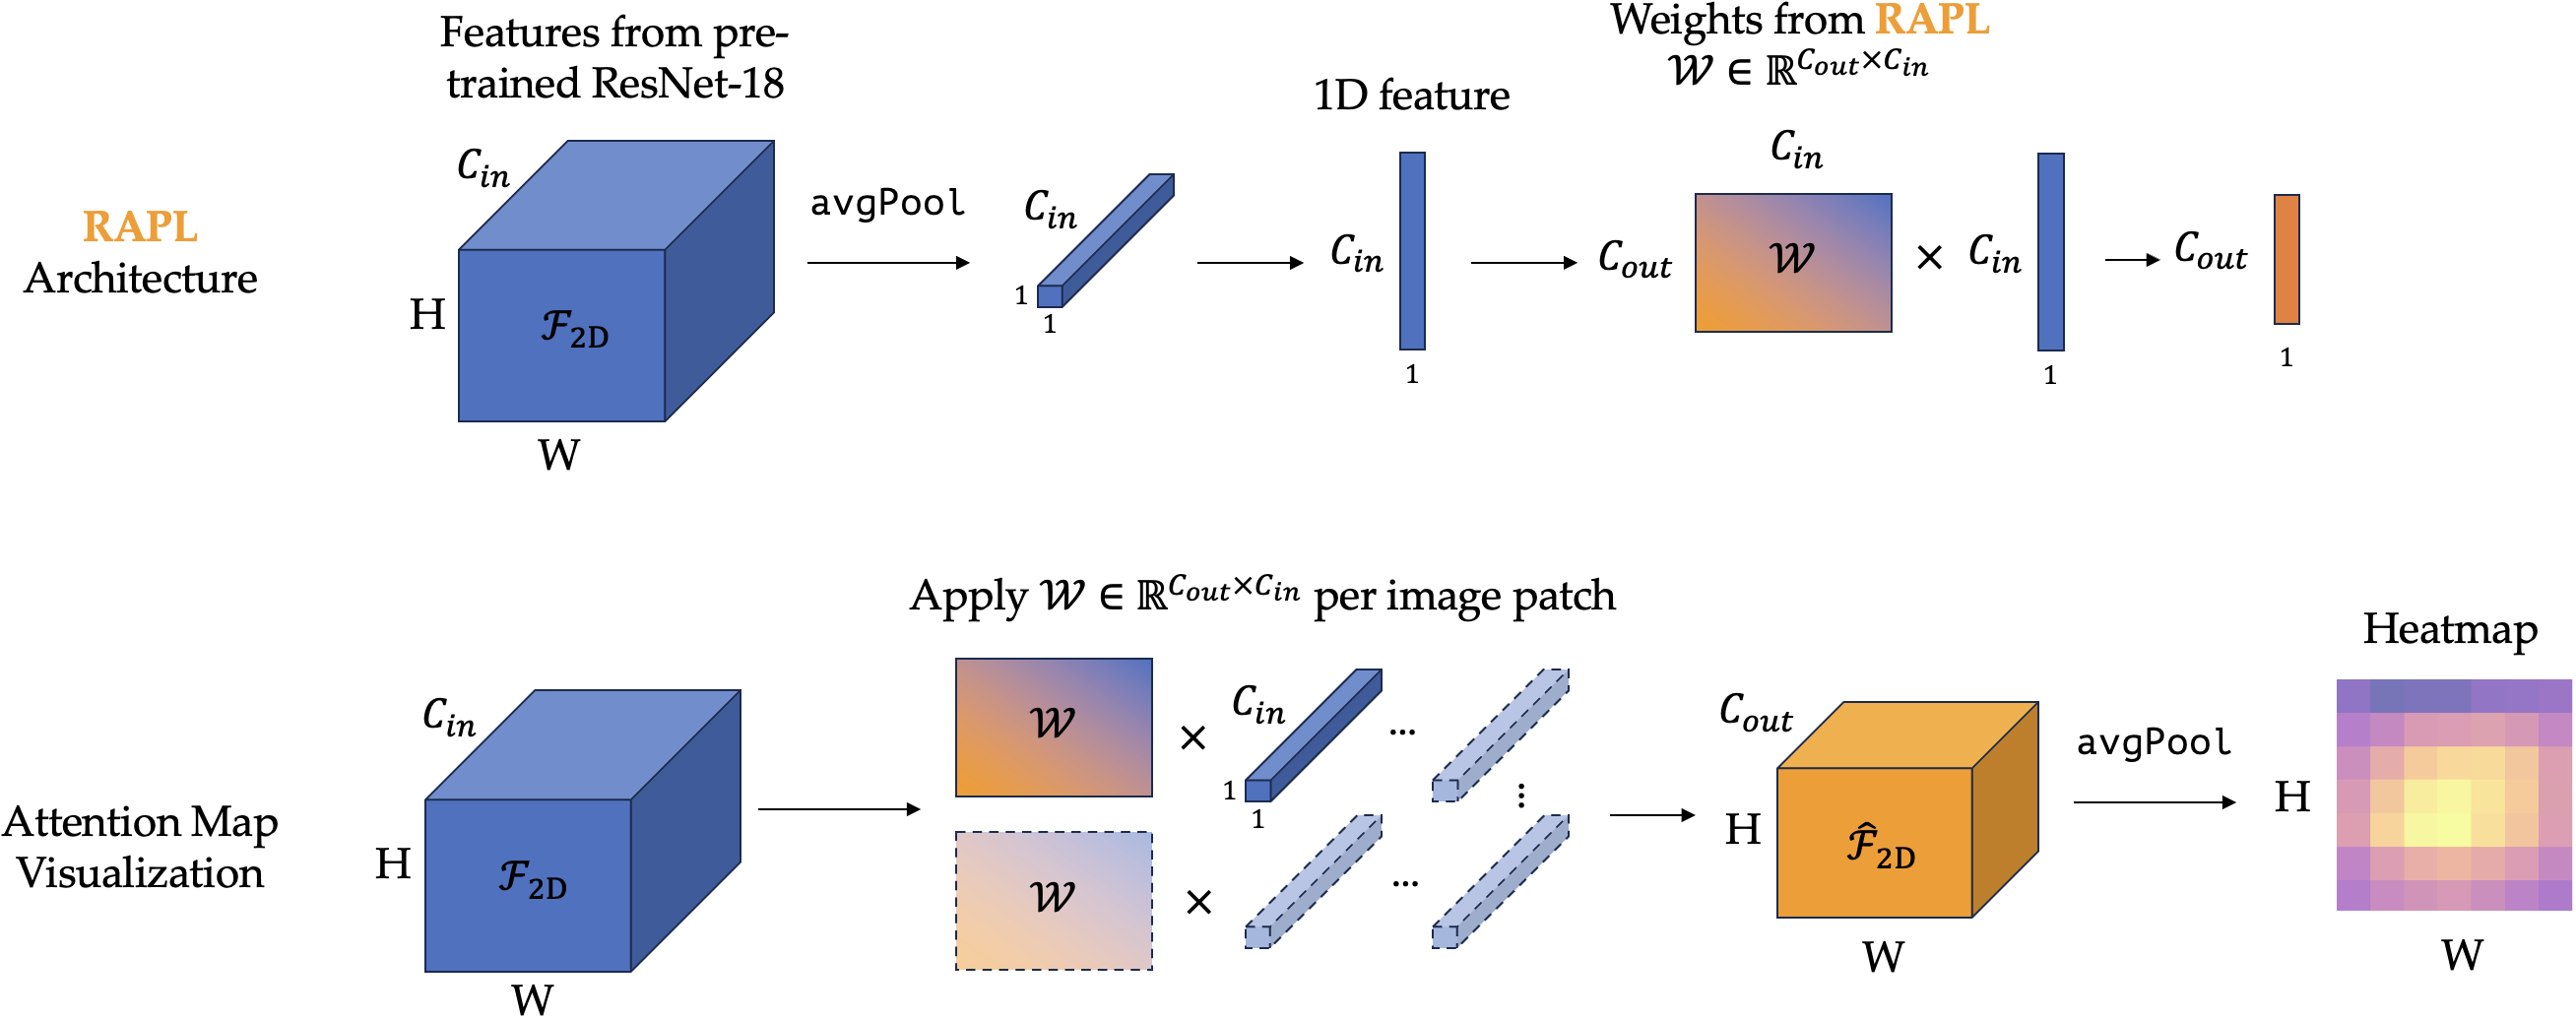}
    \caption{\rb{\textbf{Attention Map Visualization Method.} (top) Visualization of our RAPL architecture. (bottom) Visualization of our process for creating a 2D attention map.} }
    \label{fig:attention_map_method}
\end{figure*}

\subsection{Additional RLHF results: Ablation on Feedback Dataset Size}
\label{app:rlhf-with-doubled-data}

% \begin{figure}
%     \vspace{-0.0cm} 
%     \includegraphics[width=0.4\textwidth]{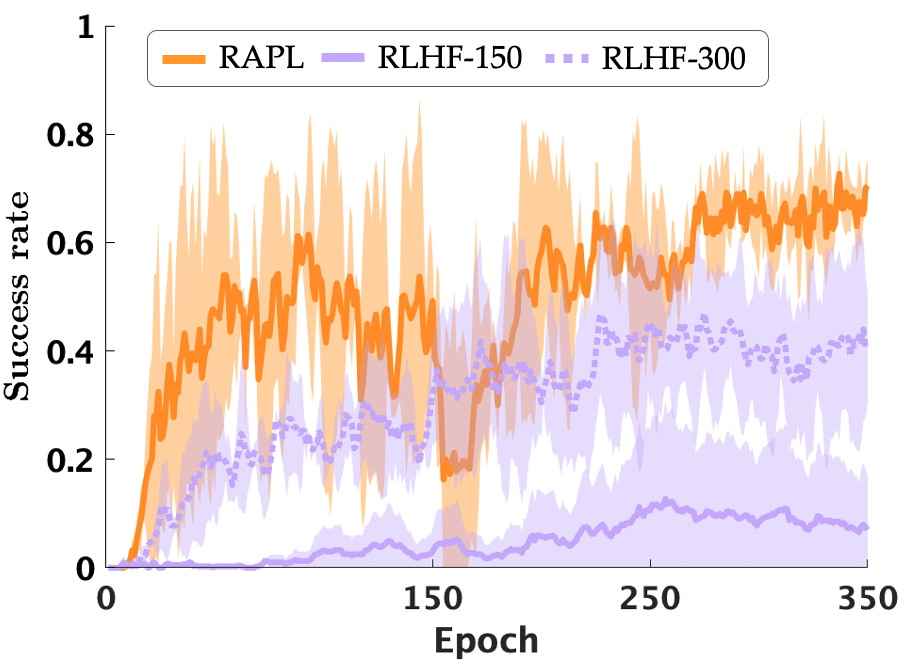}
%     \vspace{-0.5cm}
%     \caption{\textbf{Manipulation.} \rapl outperforms \rlhf by $75\%$ with $50\%$ less training data.}
%     \label{fig:rlhf_double_datasize}
%     \vspace{-0.5cm}
% \end{figure}
%
In Section~\ref{subsec:in-domain-manipulation}, it's surprising that \rlhf fails to learn a robot policy in a more realistic environment since its objective is similar to ours, but without explicitly considering representation alignment.  To further investigate this, we apply a linear probe on the final embedding and visualize the image heatmap of what \rapl's (our representation model trained with 150 training samples), \rlhf-150's (\rlhf trained with 150 samples), and \rlhf-300's (\rlhf trained with 300 samples samples) final embedding pays attention to in Figure~\ref{fig:attention_map}.

We see that $\phi_{RAPL}$ learns to focus on the objects, the contact region, and the goal region while paying less attention to the robot arm;
$\phi_{RLHF-150}$ is biased towards
paying attention to irrelevant areas
that can induce spurious correlations (such as the robot arm and background area);
$\phi_{RLHF-300}$'s attention is slightly shifted to objects while still pays high attention to the robot embodiment.

When deploying $\phi_{RLHF-300}$ in Franka manipulation policy learning, we observe that policy performance is slightly improved (indicating that with more feedback data, preference-based reward prediction could yield to an aligned policy), but \rapl still outperforms \rlhf by $75\%$ with $50\%$ less training data, supporting the hypothesis: \textit{\rapl outperforms \rlhf with lower amounts of human preference queries}.

\subsection{Additional Cross-Embodiment Results: X-Magical \& Kuka Manipulation}
\label{app:cross-domain-results}

\rb{

}

% \rb{
% \subsection{Spearman’s correlation between GT and learned visual rewards}
% \label{app: reward analysis}

% In this section, we conduct a quantitative analysis to investigate the relationship between the learned visual reward and the end-user’s ground-truth reward. Specifically, for each robot manipulation task, we compute the average Spearman’s correlation coefficient between the learned visual reward and the end-user’s ground-truth reward across 100 video trajectories. We can observe from Table~\ref{table:Spearman} that our learned visual reward shows a stronger correlation to the end-user’s ground-truth reward compared to baselines.
% {
% \renewcommand{\arraystretch}{1.5}
% \begin{table}[h!]
%     \centering
%     \begin{tabular}{p{0.6in}|c | c | c}
%        & \multicolumn{3}{|c}{ \textbf{Spearman's Correlation} } \\ \hline 
%          & \textbf{Franka Group} (Sec.~\ref{subsec:in-domain-manipulation}) & \textbf{Kuka Group} (Sec.~\ref{app:cross-domain-results}) & \textbf{Franka Clutter} (Sec.~\ref{app: multi object push}) \\\hline\hline 
%         \rapl & 0.59 &  0.47 & 0.61\\ \hline
%         \rlhf & 0.38 &  0.31 & 0.26\\ \hline
%         \mvpot &  -0.1&  0.02 & 0.08\\ \hline
%         \mvpotfinetune &  0.19&  0.02& 0.11 \\ \hline
%         \imagenet &  -0.09 &  0.12 & -0.02\\\hline
%         \rtm & 0.03 &  -0.14 &  -0.17 \\ \hline
%     \end{tabular}
%     \caption{\rb{Spearman's rank correlation coefficient between the \gt reward and each learned reward.}}
%     \label{table:Spearman}
% \end{table}
% }
% }

\newpage

\rb{
\subsection{Robot Manipulation: RLHF Perceived vs. True Success}
}

\begin{figure}
    \includegraphics[width=0.4\textwidth]{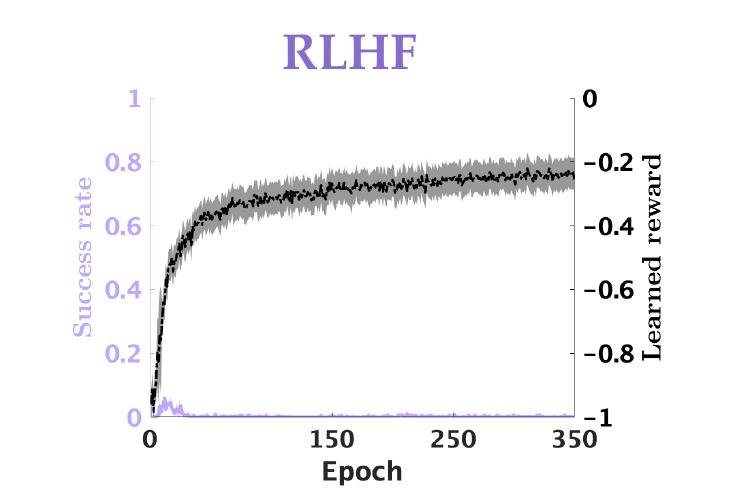}
    %\vspace{-0.8cm}
    \caption{\rb{\textbf{Manipulation.} True success rate of the RLHF policy (purple) versus the ``perceived'' performance under the RLHF reward (black).}}
    \label{fig:franka_sr_v_learnedreward_rlhf}
    %\vspace{-0.2cm}
\end{figure}
\textcolor{black}{We investigated if the poor RLHF performance in Figure~\ref{fig:franka_success_v_reward} can be attributed to poor RL optimization or to poor visual reward structure. 
We compared the true success rate of the RLHF policy (under the true human’s measure of success) to the ``perceived'' performance under the RLHF reward. 
These results are visualized in Figure~\ref{fig:franka_sr_v_learnedreward_rlhf}: purple is the true success rate and black is the ``perceived'' reward under the RLHF learned reward.
We see that after 350 epochs, the RLHF learned reward perceives the policy as achieving a high reward. However, as shown in the manuscript’s Figure~\ref{fig:franka_success_v_reward} and in Figure~\ref{fig:franka_sr_v_learnedreward_rlhf}, the true success rate is still near zero. This indicates that the RL optimization is capable of improving over time, but it is optimizing a poor reward signal that does not correlate with the true measure of success.
}
